# Supplementary material for: Fast American Option Pricing using Nonlinear Stencils
Source: arXiv:2303.02317 source file (2023-10-16)
Supplement: Supplementary file 1 [file appendix.tex]

\hide{
\subsection{Detailed Description of the Algorithm for American call option pricing under BOPM}
\label{ssec:BOPM-algo-InAppendix}

The solution space is a right-angle isosceles triangle with base length $T$. We prove the following theorem.

\begin{theorem}\label{AOT1}
There exists an algorithm that solves the American option Pricing problem with time window $T$ in $\Oh{T\log^2 T}$ time.
\end{theorem}

We present our algorithm as follows. We know the boundary between the red and green cells in the first row of the triangle (solution space), however, we do not know the locus of the boundary in the subsequent rows of the triangle. We compute the boundary in the following process. 

We partition the triangle (solution space) into trapezoids. We compute the first trapezoid with its first row as the same first row of the triangle (the solution space) and solve this newly created trapezoid (we later explain how we create a trapezoid and solve it in this section). Then we compute the second trapezoid with its first row as the last row of the first trapezoid and solve the second trapezoid. This process continues until the total height of the subsequently created trapezoids exceeds ($T-\sqrt{T}$). We will then be left with a right-angle isosceles triangle with base size at most $\sqrt{T}$. We solve this triangle iteratively by doing quadratic work in time $\Oh{T}$.

We now describe the process how we partition the solution space into trapezoids, and then how we solve each trapezoid.

\subparagraph*{\textbf{Partitioning the triangle into trapezoids.}}
 Let $abc$ be a right-angle isosceles triangle with base length $T$, as shown in Figure~\ref{img:trapezoid}. We partition triangle $abc$ in a sequence of trapezoids. Let $\ell_1$ be the number of red cells on line segment $ab$. In the American option pricing model, all the red cells in any row are consecutive. Let $\ell_1$ red cells are placed consecutively from $a$ to $p$. Let $d$ be the point on line segment $ac$ that is $\ell_1$ distance away from $a$. Draw a horizontal line from $d$; let the line intersect $bc$ at point $e$. We thus get a trapezoid $abed$ with height $\ell_1$, and the number of red cells in the first row of trapezoid $abed$ is $\ell_1$.

We solve trapezoid $abed$, and thus will know where the boundary between the red and green cells intersect line segment $de$. Let $q$ be the intersection point, and $\ell_2$ be the distance from $d$ to $q$ (solving a trapezoid means computing the values of all the red cells in the last row of the trapezoid). Let $f$ be the point on line segment $dc$ that is $\ell_2$ distance away from $d$. We draw a horizontal line $fg$, and get the second trapezoid $degf$ of height $\ell_2$. We treat the first row of the second trapezoid $degf$ as the same of the last row of the first trapezoid $abed$. 

We solve trapezoid $degf$, and thus will know where the boundary between the red and green cells intersect line segment $gf$. Let $r$ be the intersection point. We follow a similar approach to compute the subsequent trapezoids as we took to compute trapezoid $degf$. We stop this process when the total height of all the trapezoids becomes more than $(T - \sqrt{T})$. We will be left with a right-angle isosceles triangle $xyc$ with base length at most $\sqrt{T}$. We compute all the cell values of triangle $xyc$ iteratively in time $O(T)$.

In the next paragraphs, we show that a trapezoid of height $\ell$ can be solved in $O(\ell \log^2 \ell)$. Suppose that we create $k$ trapezoids using the above process. Let the heights of these $k$ trapezoids be $\ell_1, \ell_2, \ldots, \ell_k$. Summing up the running time of all the trapezoids and the triangle at the bottom, we get the total running time $\Psi$ as $
\Psi = \left( \sum_{1 \leq i \leq k}{\Oh{\ell_i \log^2 \ell_i}} \right) + \Oh{T} = \Oh{ T\log^2 T }.
%O(\ell_1 \log^2 \ell_1) + O(\ell_2 \log^2 \ell_2) + \cdots + O(\ell_k \log^2 \ell_k) + O(T) = O(T\log^2 T).
$

\subparagraph*{\textbf{Solving a trapezoid.}} We show how a trapezoid of height $\ell$ is solved as follows. Solving a trapezoid means computing the values of all the red cells in the last row of the trapezoid. We know that in the first row of the trapezoid, there are total $\ell$ red cells 
that are consecutive. Let $abcd$ be such a trapezoid of height $\ell$ where there are $\ell$ red cells from $a$ to $q$ in the first row (Figure~\ref{img:aoption}). We want to compute all the red cell values on line segment $dc$. Let $r$ be the point which is $\floor{\ell/2}$ distance away from $a$ on line segment $ad$. Draw a horizontal line from $r$; let the horizontal line intersect $bc$ at $v$. 

We compute the red cell values on $dc$ in two steps.
\begin{enumerate}
\item We compute all the red cells on line segment $rv$. 
\item Then using the cell values on line segment $rv$, we compute all the red cell values on line segment $dc$. 
\end{enumerate}

\subparagraph*{Computing the values of all red cells on line segment $rv$.}
Let line segments $rv$ and $qd$ intersect at point $t$. 
We compute the values of red cells on $rv$ in two steps. First, We compute the cell values on line segment $rt$ using the FFT-based stencil algorithm of \cite{ahmad2021fast} (all the cells on line segment $rt$ are red since the boundary between the red and green cells may move to its left at most one step per time step). Note that the lengths of both line segments $rt$ and $pt$ are the same, $\floor{\ell/2}$. The newly created trapezoid $pbvt$ has height $\floor{\ell/2}$, and there are $\floor{\ell/2}$ red cells in its first row. We solve trapezoid $pbvt$ recursively similar to trapezoid $abcd$. We thus compute all the red cell values on line segment $tv$ of trapezoid $pbvt$.

\subparagraph*{Computing the values of all red cells on line segment $dc$.}
We have already computed all the red cells on line segment $rv$. Let $u$ be the point on $rv$, such that all the cells on the left of $u$ are red and all the cells on the right of $u$ are green. Draw a line parallel to the line segment $qd$; let the line intersect $dc$ at point $w$. Next, draw a line that is perpendicular to the line segment $dc$; let the line intersect $rv$ at point $s$. 

We compute the values of all the red cells on line segment $dc$ in the following two steps.
First, We compute the cell values on line segment $dw$ using the FFT-based stencil algorithm of \cite{ahmad2021fast} (all the cells on line segment $dw$ is red since the boundary between ). Note that the lengths of both line segments $sw$ and $su$ are the same, $\ceil{\ell/2}$. The newly created trapezoid $svcw$ has height $\ceil{\ell/2}$, and there are $\ceil{\ell/2}$ red cells in its first row. We solve trapezoid $svcw$ recursively similar to trapezoid $abcd$. We thus compute all the red cell values on the line segment $wc$ of trapezoid $svcw$. 

In total, we make two calls of FFT-based periodic algorithm and solve two trapezoids $pbvt$ and $svcw$, each of height $\floor{\ell/2}$ and $\ceil{\ell/2}$. The recurrence is thus: $\zeta(\ell) = 2\zeta (\ceil{\ell/2}) + \Theta(\ell \log \ell)$. Solving this, we get $\zeta(\ell) = \Oh{\ell \log^2 \ell}$.

 \subparagraph*{Base case.}
 We can compute the base case in $\Oh{1}$ time. In the base case, there are only $\Oh{1}$ red cells in the first row of the base case trapezoid. We do not compute the green output cells and compute only the red output cells (the last row of the base trapezoid).

We use the $\max$ operator to compute the cell values in the base case. That is, in the whole computation the $\max$ operator is used only in the base case trapezoids. There are $\Oh{1}$ number of red cells in the last row of the base-case trapezoid, and these red output cells depend only on $\Oh{1}$ input cells. Hence we can compute the base case in $\Oh{1}$ time.

~\\
We will also have the following result for the parallel version of the algorithm in Theorem \ref{AOT1}:
\begin{theorem}\label{AOT2app}
    The parallel version of the algorithm in Theorem \ref{AOT1} performs $\Oh{T\log^2 T}$ work in $\Oh{ T }$ span.
\end{theorem}
\begin{proof}
    The total work of the algorithm directly follows from Theorem \ref{AOT1}. we are focusing on the span of the algorithm. We first calculate the span of calculating a trapezoid of size $\ell$. Recall that we can solve trapezoid $svcw$ only after solving trapezoid $pbvt$. However, we can run the FFT-based algorithm for computing $rt$ in parallel with the recursive call for solving 
    $pbvt$, and the FFT-based algorithm for computing $dw$ in parallel with the recursive call for solving $svcw$.
    Hence, the total span of this part will be $\Oh{\log \ell \log \log \ell}$ \cite{ahmad2021fast}. Denote by $\zeta_{\infty}$ the total span of solving a trapezoid of size $\ell$. Then, we will have $\zeta_{\infty}(\ell) = 2 \zeta_{\infty} (\ceil{\ell/2}) + \Oh{\log \ell \log  \log \ell}$. 
    Thus $\zeta_{\infty}(\ell) = \Oh{\ell}$. Since the trapezoid of size $\ell_1,\ell_2,\cdots,\ell_k$ are calculated in serial, the total span of solving all the trapezoid $\Psi_{\infty}$ is $
    \Psi_{\infty} = \Oh{ \ell_1 } + \Oh{ \ell_2 } + \cdots + \Oh{ \ell_k } + \Oh{\sqrt{T}} = \Oh{T}.$ Hence, we complete the proof of the theorem.
\end{proof}
%Let line segments $qd$ and $rv$ intersect at point $t$. We compute all the red cell values on line segment $rv$. We know that all the cells on line segment $rt$ are red. We compute all cells on $rt$ by doing a periodic FFT algorithm. 

% \begin{algorithm}
% \small
% \caption{American Option Pricing}\label{alg:op-ame}
% \KwData{An array $A$ of possible prices in the future.}
% \KwResult{The option price.}
%     \begin{algorithmic}[1]
%     % \Comment{\textbf{TODO here}}
%     % \State $C \gets \sum_{\bm{x}}S[\bm{x}, \bm{0}]$
%     % \State $S_n[\bm{x}, \bm{0}] \gets S[\bm{x}, \bm{0}] \times C^{-1}, \forall \bm{x}$
%     Find the boundary point for $A$ and the index to be $l$. 
%     We can calculate $\frac{l}{2}$ using FFT.
%     until reaching  constant number of  cell.
%     \end{algorithmic} 
% \end{algorithm}
}
% hide ends

% \input{Arxiv/trinomial/trinomial}
%\input{Arxiv/trinomial/TOPM}
